# Supplementary material for: MemWarp: Discontinuity-Preserving Cardiac Registration with Memorized Anatomical Filters
Source: arXiv:2407.08093 source file (2024-07-10)
Supplement: Supplementary file 1 [file appendix.tex]

\section{Appendix}
